# Supplementary material for: ESPN: Extremely Sparse Pruned Networks
Source: arXiv:2006.15741 source file (2020-06-28)
Supplement: Supplementary file 1 [file appendix.tex]

\appendix

\newpage 
